# Supplementary material for: The Importance of Suppressing Domain Style in Authorship Analysis
Source: arXiv:2005.14714 source file (2020-05-29)
Supplement: Supplementary file 1 [file domain-style-appendices.tex]

\appendix

\begin{center}
\Large
{\bf Supplementary Material}

\medskip
\normalsize
for ``Adversarial Training for Domain-Invariant Writing Style Representations''

\medskip
\small
(the Appendix will be added to the paper on publication)
\end{center}

\section{Data}

From March 21 to July 2nd 2018, we downloaded every single story from fanfiction.net that was available at the time (latest available story id: 12~987~600). Some stories consists of several chapters, and for each chapter, there is a corresponding HTML file. In total, we downloaded 26,424,126 single HTML files. These had to be filtered first, because some files turned out to contain only error messages saying that the particular chapter was not available any longer. Moreover, we decided to exclude stories from the ``Crossover'' and ``Misc'' categories. Crossovers are fanfictions whose plot is connected with more than one fandom and therefore has more than just one topic label. The Misc category happens to also include crossovers, which is why they were filtered out as well. After this filtering step, we still had 24,390,714 HTML files available, corresponding to 5,800,292 usable stories in 44 languages from 1,400,958 authors writing in 10,328 different fandoms (= topics). Additionally, the HTML files include meta information about genre (e.g., ``Romance''), number of reviews, number of times favourited by another user, etc. We parsed the text using the BeautifulSoup 4 package for Python. Since our goal was to extract a ``pure'' representation of each author's writing style, we tried to remove any artefactual traces that a model could use to overfit on author. First, in-text headlines (denoted by \lstinline|<h1>| and \lstinline|<h2>| html tags) were removed. This was done since many authors include own chapter or subchapter headlines in their stories. Second, centered paragraphs were removed, as they were found to frequently include text that is neither relevant to the story nor part of it, such as acknowledgements. The same applies to paragraphs written fully in bold or underlined text. Then, the first paragraph or the first five percent of the text, whatever is more, was removed. The text was always cut at the end of a sentence. The same procedure was applied to the last paragraph / the last five percent of the text. This was done because we noticed that the first and last parts of a chapter often contain information that are not part of the actual stories (e.g. claims of authorship and / or copyright).

\begin{table}[tb]%
\centering%
\small%
\renewcommand{\tabcolsep}{1pt}%
\begin{tabular}{@{}l@{\kern-0.5em}r@{}r@{\ \ }rrr@{}}
\toprule
\bf Language & \bf Stories\ \ \null & \bf Fandoms & \multicolumn{3}{@{}c@{}}{\bf Text Length (Characters)} \\
\cmidrule(r@{\tabcolsep}){4-6}\cmidrule(l@{\tabcolsep}){4-6}
& & & Avg. & Std. Dev. & Max. \\
\midrule
English    & 5,098,568  & 10,012 & 53,015 & 179,701 & 216,007,457 \\
Spanish    & 320,272    & 3,101  & 66,365 & 184,807 & 16,050,508  \\
French     & 148,761    & 2,397  & 76,721 & 204,072 & 8,074,334   \\
Indonesian & 108,290    & 1,418  & 43,785 & 95,669  & 5,356,883   \\
Portuguese & 68,908     & 1,454  & 59,054 & 163,997 & 7,069,225   \\
German     & 27,227     & 987    & 80,506 & 225,056 & 10,688,021  \\
Russian    & 8,668      & 378    & 50,342 & 163,651 & 5,635,119   \\
Italian    & 3,883      & 395    & 53,526 & 154,042 & 3,600,036   \\
Hungarian  & 2,076      & 259    & 70,967 & 211,417 & 4,506,201   \\
\bottomrule
\end{tabular}%
\caption{Corpus statistics by text language}
\label{table-corpus-statistics}%
\end{table}

Furthermore, strings containing repeating character patterns ("$\sim$+$\sim$+$\sim$+$\sim$+$\sim$") often used for demarcation were deleted, as well as * signs. The latter were sometimes used by authors at the start of each of their sentences. It was also made sure to attain a unified quotation string, all quotation characters (backticks, forwardticks, double quotes) were replaced by a single quote sign. Finally, paragraphs that begin with the word "disclaimer" or "dedication" and are followed by a colon were removed. We performed this text cleaning with much attention to detail and according to the best of our knowledge and belief. Given the vast nature of the corpus, we certainly could not get rid of every single artefact, but we may assume the rest of noise to be negligible.

%%% ADDITION.
% \input{table-author-intersection}

\section{Models}

Where we do not state anything else, we use the standard parameters of tensorflow 1.12.0~\cite{abadi:2016} and scikit-learn 0.20~\cite{scikit-learn}.

\subsection{SVM, Random Forest and Na\"ive Bayes}

SVM, Random Forest and Na\"ive Bayes were trained with scikit-learn with random search hyperparameter tuning including 3-fold cross validation. For the SVM, optimized parameters included kernel, gamma, C, and degree. 60 different parameter combinations are tested with an increased cache size of 2GB and stopping of the optimization after maximal 10000 iterations. For the Random Forest, we optimized n\_estimators, max\_depth, min\_samples\_split, max\_features, bootstrap, and criterion. Finally, for Naive Bayes the optimized parameters included alpha and fit\_prior.

\subsubsection{Neural Network Trained on 2 Authors}

LSTM layer with 256 units - 2x fully connected layer with 64 neurons and ReLU activation function - [Author prediction: 1x fully connected layer with 64 neurons and ReLU activation function | Fandom prediction: 1x fully connected layer with 64 neurons and ReLU activation function]

Dropout of 50\% applied on fully connected layer of author prediction and fandom prediction, Adam optimizer with learning rate $10^{-5}$, batch normalization, mini-batch size 400 and random seed 1.

\subsubsection{Neural Network Trained on 10 Authors}

LSTM layer with 256 units - 2x fully connected layer with 64 neurons and ReLU activation function - [Author prediction: 1x fully connected layer with 64 neurons and ReLU activation function | Fandom prediction: 1x fully connected layer with 64 neurons and ReLU activation function]

Dropout of 50\% applied on fully connected layer of author prediction and fandom prediction, Adam optimizer with learning rate $10^{-3}$, batch normalization, mini-batch size 400 and random seed 1.
